# Supplementary material for: Linear Semantic Segmentation for Low-Resource Spoken Dialects
Source: arXiv:2605.06276 source file (2026-05-07)
Supplement: Supplementary file 1 [file plots.tex]

\section{WD performance across data sources}
\label{sec:appendix-figures}

\noindent
\includegraphics[width=\textwidth,
                 height=0.4\textheight,
                 keepaspectratio]{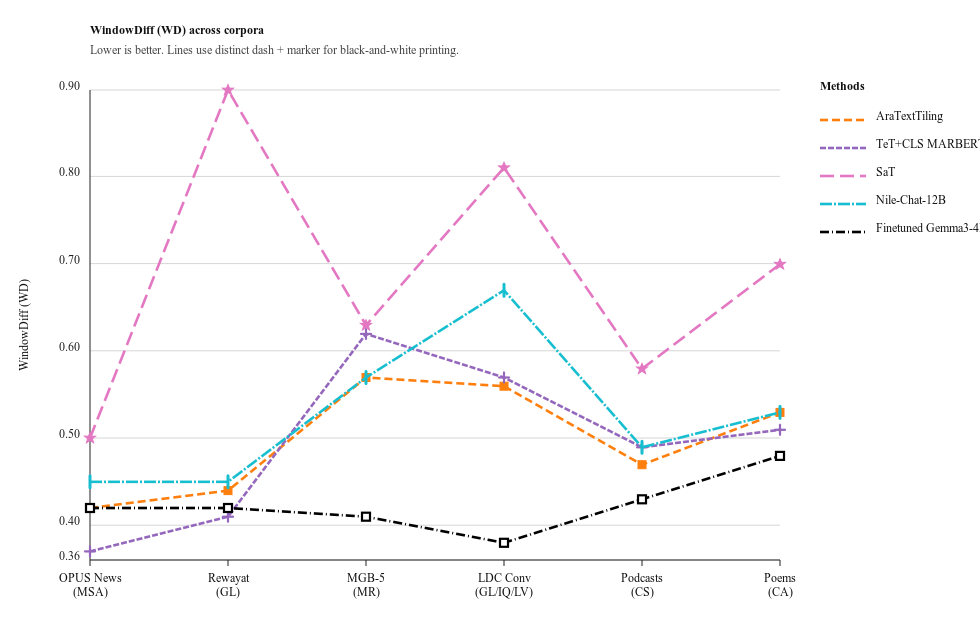}

\medskip

\noindent
\includegraphics[width=\textwidth,
                 height=0.4\textheight,
                 keepaspectratio]{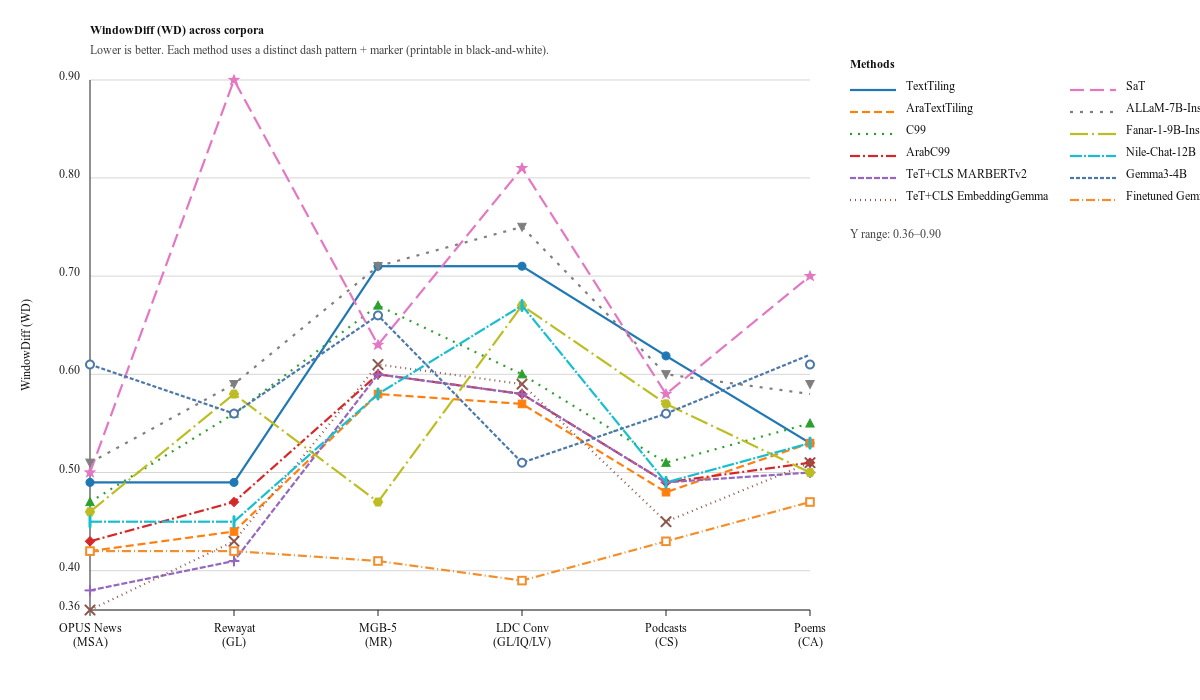}
